# Supplementary material for: Nuclear Quantum Effects on Autoionization of Water Isotopologues Studied by Ab Initio Path Integral Molecular Dynamics
Source: arXiv:2101.12500 source file (2021-01-29)
Supplement: Supplementary file 1 [file SuppInfo.pdf]

# Supplementary Material: Nuclear Quantum Effects on Autoionization of Water Isotopologues Studied by Ab Initio Path Integral Molecular Dynamics

Bo Thomsen[1, a)] and Motoyuki Shiga[1, b)]
*CCSE, Japan Atomic Energy Agency, 178-4-4, Wakashiba, Kashiwa, Chiba, 277-0871, Japan*

(Dated: 28 January 2021)

[a)] Electronic mail: thomsen.bo@jaea.go.jp
[b)] Electronic mail: shiga.motoyuki@jaea.go.jp

Table SI. Autoionization constants of water isotopologues calculated by the probabilistic method using the experimental p$K_W$ of $D_2O$ to calculate $R_c$.

| Method | System | Molecules | $P$ | p$K_W$ (PROB) | $R_c$ [Å] |
|---|---|---|---|---|---|
| DFT[a] | liq. $H_2O$ | 32 | 12 | 15.4 ± 0.9 | 1.53±0.04 |
| DFT[a] | liq. $D_2O$ | 32 | 12 | 14.9[d] | 1.53±0.04 |
| DFT[a] | liq. $T_2O$ | 32 | 12 | 16.2 ± 0.8 | 1.53±0.04 |
| DFTB[b] | liq. $H_2O$ | 32 | 12 | 13.9 ± 0.3 | 1.16±0.00 |
| DFTB[b] | liq. $D_2O$ | 32 | 12 | 14.9[d] | 1.16±0.00 |
| DFTB[b] | liq. $T_2O$ | 32 | 12 | 14.9 ± 0.2 | 1.16±0.00 |
| OSS2[c] | liq. $H_2O$ | 64 | 12 | 13.6 ± 0.4 | 1.51±0.02 |
| OSS2[c] | liq. $D_2O$ | 64 | 12 | 14.9[d] | 1.51±0.02 |
| OSS2[c] | liq. $T_2O$ | 64 | 12 | 14.9 ± 0.7 | 1.51±0.02 |

[a]Ab initio PIMD.
[b]Semiempirical PIMD.
[c]Empirical PIMD.
[d]Reference value to determine $R_c$.

Table SII. Autoionization constants of water isotopologues calculated by the absolute method

| Method | System | Molecules | $P$ | p$K_W$ (ABS) |
|---|---|---|---|---|
| DFTB[a] | liq. $H_2O$ | 32 | 1 | 46.3 ± 0.7 |
| DFTB[b] | liq. $H_2O$ | 32 | 12 | 43.8 ± 0.8 |
| DFTB[b] | liq. $D_2O$ | 32 | 12 | 43.2 ± 0.8 |
| DFTB[b] | liq. $T_2O$ | 32 | 12 | 44.5 ± 0.6 |
| DFTB[b] | liq. $H_2O$ | 32 | 32 | 43.9 ± 0.8 |
| DFTB[b] | liq. $T_2O$ | 32 | 32 | 43.5 ± 0.6 |
| DFTB[a] | liq. $H_2O$ | 64 | 1 | 45.8 ± 0.3 |
| DFTB[b] | liq. $H_2O$ | 64 | 12 | 44.2 ± 0.4 |
| DFTB[b] | liq. $T_2O$ | 64 | 12 | 44.4 ± 0.5 |

[a]Semiempirical MD.
[b]Semiempirical PIMD.
